# Supplementary material for: Structured Temporal Causality for Interpretable Multivariate Time Series Anomaly Detection
Source: arXiv:2510.16511 source file (2026-10-21)
Supplement: Supplementary file 1 [file title.tex]

\makeatletter

% Define the appendix title box
\newcommand{\NIPStitle}[1]{%
  \clearpage
  \vbox{%
    \hsize\textwidth
    \linewidth\hsize
    \vskip 0.1in
    \@toptitlebar
    \centering
    {\LARGE\bfseries #1\par}
    \@bottomtitlebar
    \vskip 0.2in
  }%
}

\makeatother

\clearpage

\newpage
\appendix
\onecolumn

% \part*{Appendix}
\setcounter{equation}{0}
\setcounter{figure}{0}
\setcounter{table}{0}
\setcounter{footnote}{0}

\makeatletter

\NIPStitle{Appendix for "Structured Temporal Causality for Interpretable
Multivariate Time Series Anomaly Detection"}
